# Supplementary material for: High order geometric methods with splines: an analysis of discrete Hodge--star operators
Source: arXiv:2203.00620 source file (2022-07-15)
Supplement: Supplementary file 3 [file appendix.tex]

%\noindent {\color{blue} \textbf{Assigned Author(s):} Vazquez and Evans}\\

%\noindent {\color{blue} \textbf{Synopsis:} I vote to place as many of the technical details as we possibly can in this appendix.  In fact, I would contend we simply state the final result in the text of the paper, and we relegate the remainder of the necessary lemmas and final results to the appendix.  This will yield a long appendix, but I fear the details may actually interfere with the other details of the paper.}

%\appendix
%%%%%%%%%%%%%%%%%%%%%%%%%%%%%%%%%%%%%%%%%%%%%%%%%%%%%%%%%%%%
\section{Proof of Theorem~\ref{th:homology}}\label{sec:appendix}
%%%%%%%%%%%%%%%%%%%%%%%%%%%%%%%%%%%%%%%%%%%%%%%%%%%%%%%%%%%%

Without loss of generality, we assume that the polynomial degree is the same in both parametric directions (i.e., $p = p_1 = p_2$) as this greatly simplifies our exposition. However, the subsequent analysis also holds in the mixed polynomial degree setting.

Let us begin by recalling notation from the main text. We denote the B\'ezier meshes of two consecutive levels $\ell$ and $\ell+1$ by $\M_{\ell}$ and $\M_{\ell+1}$, respectively, and we denote the Greville subgrids of two consecutive levels by $\MG_{\ell}$ and $\MG_{\ell+1}$.  For the subdomain $\Omega_{\ell+1}$ appearing in the hierarchical B-spline construction, we denote the corresponding B\'ezier submeshes associated with levels $\ell$ and $\ell+1$ by $\M_{\ell,{\ell+1}} \subset \M_\ell$ and $\M_{\ell+1,{\ell+1}} \subset \M_{\ell+1}$. We further denote the Greville subgrids associated with functions whose support is completely contained in $\Omega_{\ell+1}$ for levels $\ell$ and $\ell+1$ by $\MG_{\ell,\ell+1} \subset \MG_\ell$ and $\MG_{\ell+1,\ell+1} \subset \MG_{\ell+1}$. With some abuse of notation, the subdomains occupied by the Greville subgrids are also denoted by $\MG_{\ell,\ell+1}$ and $\MG_{\ell+1,\ell+1}$.

We now establish some additional definitions that will be required in our subsequent analysis.  Given a B\'ezier element $Q \in \M_{\ell}$, we define the extended support\footnote{This has been traditionally denoted by $\tilde Q$ in the IGA literature.}, denoted as $\M_{\ell,\tilde Q} \subset \M_\ell$, to be the union of the support of basis functions in ${\cal B}^k_\ell$ that do not vanish in $Q$, for $k = 0, 1, 2$. We define a corresponding Greville subgrid, denoted as $\MG_{\ell,\tilde Q} \subset \MG_\ell$, to be that formed by the vertices, edges, and cells of the Greville grid $\MG_\ell$ associated with basis functions that do not vanish in $Q$. 
%Notice the slight abuse of notation, since in the case of low regularity there may be functions completely supported in $\tilde Q$ such that their geometrical entities are not in $\MG_{\ell,\tilde Q}$.
Finally, we define an additional Greville subgrid $\MG'_{\ell,\tilde Q}$ to be the extension of $\MG_{\ell,\tilde Q}$ obtained by adding one cell in each direction (see Figure~\ref{fig:qtilde}), noting that when $\MG_{\ell,\tilde Q}$ is adjacent to the boundary the extension in the corresponding direction is not necessary.  It should be noted that the Greville subgrids $\MG_{\ell,\tilde Q}$ and $\MG'_{\ell,\tilde Q}$ are not related to the previously defined Greville subgrids $\MG_{\ell,\ell+1}$ and $\MG_{\ell+1,\ell+1}$.

%It is also worth to note that, in general, for an element $Q \in \M_{\ell,\ell+1}$ these subgrids are not necessarily contained in $\M_{\ell,\ell+1}$ and $\MG_{\ell,\ell+1}$, respectively.

\begin{figure}[t]
\begin{subfigure}[Element $Q$ and its extended support $\M_{\ell,\tilde Q}$.]{
\includegraphics[width=0.48\textwidth]{MB_qtilde}
}
\end{subfigure}
\begin{subfigure}[Greville subgrids $\MG_{\ell,\tilde Q}$ (solid) and $\MG'_{\ell,\tilde Q}$ (solid and dashed).]{
\includegraphics[width=0.48\textwidth]{MG_qtilde}
}
\end{subfigure}
\caption{Extended support for an element in the B\'ezier mesh and the corresponding Greville subgrids for degree $p=5$.} \label{fig:qtilde}
\end{figure}

The following lemma states two geometrical results for B\'ezier and Greville grids.
\begin{lemma} \label{lemma:one-cell} The following statements hold:
\begin{enumerate}[i)]
\item For any Greville cell $K \in \MG_{\ell}$, with $\beta_K \in {\cal B}^2_\ell$ the corresponding basis function, it holds that $K \subset \supp(\beta_K)$.
\item For any B\'ezier element $Q \in \M_{\ell}$, it holds that $Q \subset \MG_{\ell,\tilde Q}$.
\end{enumerate}
\end{lemma}
\begin{proof}
It is sufficient to prove the result in the univariate setting of Section~\ref{sec:univariate} since the multivariate case is proved by Cartesian product.
\begin{enumerate}[i)]
\item Given two consecutive Greville points $\gamma_i = \frac{\xi_i + \ldots + \xi_{i+p-1}}{p} \ge \xi_i$ and $\gamma_{i+1} = \frac{\xi_{i+1} + \ldots + \xi_{i+p}}{p} \le \xi_{i+p}$, the basis function associated to the edge between them is $D_{i,p-1}$, which is supported in the interval $(\xi_i,\xi_{i+p})$.  Since $(\xi_i,\xi_{i+p}) \subseteq (\gamma_i,\gamma_{i+p})$, the desired result follows.
\item Given the non-empty element $(\xi_i, \xi_{i+1})$, its extended support is the interval $(\xi_{i-p}, \xi_{i+p+1})$, and the first and last basis functions that do not vanish in the element are associated to the Greville points $\gamma_{i-p+1} = \frac{\xi_{i-p+1} + \ldots + \xi_i}{p} \le \xi_i$ and $\gamma_{i+1} = \frac{\xi_{i+1} + \ldots + \xi_{i+p}}{p} \ge \xi_{i+1}$.
\end{enumerate}
\end{proof}

In what follows, we index the elements in the extended support $\M_{\ell,\tilde Q}$ from $1$ to $2p+1$ in each direction (including empty elements), the cells in the Greville subgrid $\MG_{\ell,\tilde Q}$ from 1 to $p$ in each direction, and the cells in $\MG'_{\ell,\tilde Q}$ from 0 to $p+1$ in each direction.  This is graphically depicted in Figure~\ref{fig:qtilde}. The support of the function in ${\cal B}^2_\ell$ corresponding to the cell $K_{i,j}$ in $\MG'_{\ell,\tilde Q}$ is given by the elements $\{Q_{k_1,k_2} \in \M_{\ell,\tilde Q} : i+1 \le k_1 \le i+p, j+1 \le k_2 \le j+p\}$. The following lemma states that, if two cells of $\MG_{\ell,\tilde Q}$ in the same row (column) belong to $\MG_{\ell,\ell+1}$, all the cells of the row (column) between them also belong to $\MG_{\ell,\ell+1}$.  That is, the supports of all the functions associated with cells in the row (column) are contained in $\Omega_{\ell+1}$. The proof, which we omit, is an immediate consequence of the support characterization above.

\begin{lemma} \label{lemma:supp}
Let $Q \in \M_{\ell,\ell+1}$ and further let $K_{i,j} \in \MG_{\ell,\tilde Q} \cap \MG_{\ell,\ell+1}$ where $i$ and $j$ are local indices as discussed above. If $K_{i,j_0} \in \MG'_{\ell,\tilde Q} \cap \MG_{\ell,\ell+1}$, then $K_{i,k} \in \MG_{\ell,\ell+1}$ for $\min\{j,j_0\} \le k \le \max\{j,j_0\}$. Analogously, if $K_{i_0,j} \in \MG'_{\ell,\tilde Q} \cap \MG_{\ell,\ell+1}$, then $K_{k,j} \in \MG_{\ell,\ell+1}$ for $\min\{i,i_0\} \le k \le \max\{i,i_0\}$.
\end{lemma}

With the previous definitions and results, we are now in a position to prove Theorem~\ref{th:homology}. The principal idea is to establish one-to-one correspondences between the connected components and holes of the subdomain $\Omega_{\ell+1}$ and those of the regions defined by the Greville subgrids $\MG_{\ell,\ell+1}$ and $\MG_{\ell+1,\ell+1}$. We begin with the connected components.

\begin{proposition}\label{prop:cc}
The following statements hold:
\begin{enumerate}[i)]
\item Every connected component of $\MG_{\ell,\ell+1}$ is contained in a connected component of $\MG_{\ell+1,\ell+1}$.
\item Every connected component of $\MG_{\ell+1,\ell+1}$ is contained in a connected component of $\Omega_{\ell+1}$.
\item Under Assumptions~\ref{ass:support} and~\ref{ass:overlap}, every connected component of $\Omega_{\ell+1}$ contains exactly one connected component of $\MG_{\ell,\ell+1}$.
\end{enumerate}
\end{proposition}
\begin{proof}
We prove each statement independently.
\begin{enumerate}[i)]
\item It suffices to show that each cell in $\MG_{\ell,\ell+1}$ is contained in a connected component of $\MG_{\ell+1,\ell+1}$. Let $K \in \MG_{\ell,\ell+1}$ denote a Greville cell and let $\beta_K \in {\cal B}^2_\ell$ its associated basis function.  By the nestedness of spline refinement, we note that $\beta_K$ can be expressed in terms of basis functions associated with level $\ell + 1$.  That is, we can write $\beta_K$ uniquely as: $$\beta_K = \sum_{\beta' \in {\cal B}^2_{\ell+1}} c_{\beta'} \beta'$$
where $c_{\beta'} \in \mathbb{R}$ for all $\beta' \in {\cal B}^2_{\ell+1}$.  We refer to those functions $\beta' \in {\cal B}^2_{\ell+1}$ for which $c_{\beta'} \neq 0$ as the children of $\beta_K$.  As the B-spline basis functions in ${\cal B}^2_{\ell+1}$ are non-negative and form a partition of unity, it holds that the coefficients $c_{\beta'}$ are all non-negative, and the coefficients associated with the children are all positive.  It follows that the children of $\beta_K$ are fully supported within the support of $\beta_K$.  Since $\beta_K$ is completely supported in $\Omega_{\ell+1}$, all the children of $\beta_K$ are also supported in $\Omega_{\ell+1}$. Consequently, the Greville cells associated with the children of $\beta_K$ belong to $\MG_{\ell+1,\ell+1}$. It is easily shown that the closure of the union of the Greville cells associated with the children of $\beta_K$ contains $K$ and is connected, thus the desired result follows.

\item The result is a trivial consequence of point i) in Lemma~\ref{lemma:one-cell}.
\item The arguments of the proof work for each connected component of $\Omega_{\ell+1}$, so we can assume without loss of generality that $\Omega_{\ell+1}$ is connected. The existence of a connected component of $\MG_{\ell,\ell+1}$ contained in $\Omega_{\ell+1}$ is an immediate consequence of Assumption~\ref{ass:support} and the previous two points of this proposition. The proof of uniqueness, instead, is rather technical.

Let us assume that uniqueness does not hold and, without loss of generality, that there are only two connected components of $\MG_{\ell,\ell+1}$ which we denote by $C_1$ and $C_2$. With some abuse of notation, we denote by $\supp(C_k)$ the union of the supports of the basis functions associated to the entities (vertices, edges, cells) in $C_k$ and by
 $\supp (\overline{C_k})$ the union of the supports considering also the entities on the boundary of $C_k$.  By construction, $\supp (\overline{C_k})$ contains one more element in each direction than $\supp(C_k)$.
%
By Assumption~\ref{ass:support}, we know that $\Omega_{\ell+1}$ is covered by $\supp(C_1) \cup \supp(C_2)$, and since $\supp(C_1) \cup \supp(C_2)$ is connected, there is at least one B\'ezier element $Q \subset \supp(C_1) \cap \supp(\overline{C_2})$\footnote{With more connected components, for each $C_i$ there exists a $C_j$ such that the intersection in one element holds true.}. As a consequence, there exists at least one Greville cell $K_1 \subset C_1$ such that $K_1 \subset \MG_{\ell,\tilde Q}$ and another Greville cell $K_2 \subset C_2$ such that $K_2 \subset \MG'_{\ell,\tilde Q}$. We will prove that Lemma~\ref{lemma:supp} and Assumption~\ref{ass:overlap} prevent the coexistence of two such cells, resulting in a contradiction.

To proceed forward, we establish some terminology using the index notation introduced earlier.  Let $i_{left}$ and $i_{right}$ denote the column indices associated with the leftmost and rightmost Greville cells, respectively, of $C_1 \cap \MG_{\ell,\tilde Q}$, and let $j_{bottom}$ and $j_{top}$ denote the row indices associated with the bottommost and topmost Greville cells of $C_1 \cap \MG_{\ell,\tilde Q}$.  Then, either one of the following two properties hold:
\begin{enumerate}
\item The Greville cell $K_2 \subset C_2$ satisfies $K_2 = K_{i_2,j_2}$ with $i_{left} \leq i_2 \leq i_{right}$ or $j_{bottom} \leq j_2 \leq j_{top}$.
\item The Greville cell $K_2 \subset C_2$ satisfies $K_2 = K_{i_2,j_2}$ with either $i_2 < i_{left}$ or $i_2 > i_{right}$, and also $j_2 < j_{bottom}$ or $j_2 > j_{top}$.
\end{enumerate}

%% \begin{enumerate}
%% \item The Greville cell $K_2 \subset C_2$ satisfies $K_2 = K_{i_2,j_2}$ with $i_{left} \leq i_2 \leq i_{right}$ and $j_{bottom} \leq j_2 \leq j_{top}$.
%% \item The Greville cell $K_2 \subset C_2$ satisfies $K_2 = K_{i_2,j_2}$ with at least one of $i_2 < i_{left}$, $i_2 > i_{right}$, $j_2 < j_{bottom}$, $j_2 > j_{top}$.
%% \end{enumerate}

Let us assume first that property (a) listed above holds, and in particular that $K_2 = K_{i_2,j_2}$ with $i_{left} \leq i_2 \leq i_{right}$, the other case being analogous.  Since $i_{left} \leq i_2 \leq i_{right}$ and $C_1 \cap \MG_{\ell,\tilde Q}$ is connected, we know that there exists a $j*$ such that $j_{bottom} \leq j* \leq j_{top}$ and $K_{i_2,j*} \in C_1 \cap \MG_{\ell,\tilde Q}$.  By Lemma~\ref{lemma:supp}, we can then form a column of Greville cells in $\MG_{l,l+1}$ from $K_2 = K_{i_2,j_2}$ to $K_{i_2,j*}$, and as a consequence, $C_1$ and $C_2$ are connected in contradiction with our earlier assumption.

%% Let us assume first that property (a) listed above holds.  Then $K_2 = K_{i_2,j_2}$ with $i_{left} \leq i_2 \leq i_{right}$ and $j_{bottom} \leq j_2 \leq j_{top}$.  Since $i_{left} \leq i_2 \leq i_{right}$ and $C_1 \cap \MG_{\ell,\tilde Q}$ is connected, we know that there exists a $j*$ such that $j_{bottom} \leq j* \leq j_{top}$ and $K_{i_2,j*} \in C_1 \cap \MG_{\ell,\tilde Q}$.  By Lemma~\ref{lemma:supp}, we can then form a column of Greville cells in $\MG_{l,l+1}$ from $K_2 = K_{i_2,j_2}$ to $K_{i_2,j*}$, and as a consequence, $C_1$ and $C_2$ are connected in contradiction with our earlier assumption. 

Let us now assume that property (b) holds.  More specifically, let us assume that $K_2 = K_{i_2,j_2}$ with $i_2 < i_{left}$ and $j_2 < j_{bottom}$, the other three cases being analogous.  The Greville cells of $C_1 \cap \MG_{\ell,\tilde Q}$ whose row index is $i_{left}$ are the leftmost cells of $C_1 \cap \MG_{\ell,\tilde Q}$, and by Lemma~\ref{lemma:supp}, these cells form a single column.  Consequently, we may denote these cells by $K_{i_{left},j}$ with $j_* \le j \le j^*$, and in particular $j_2 < j_{bottom} \le j_*$.

%% Let us now assume that property (b) holds.  More specifically, let us assume that $K_2 = K_{i_2,j_2}$ with $i_2 < i_{left}$.  The Greville cells of $C_1 \cap \MG_{\ell,\tilde Q}$ whose row index is $i_{left}$ are the leftmost cells of $C_1 \cap \MG_{\ell,\tilde Q}$, and by Lemma~\ref{lemma:supp}, these cells form a single column.  Consequently, we may denote these cells by $K_{i_{left},j}$ with $j_* \le j \le j^*$.  By Lemma~\ref{lemma:supp}, we cannot have that $j_* \le j_2 \le j^*$, otherwise $C_1$ and $C_2$ would be connected.  Thus, either $j_2 < j_*$ or $j_2 > j^*$.  We assume moving forward that $j_2 < j_*$ as the case $j_2 > j^*$ may be handled in an analogous manner.

Consider the cells $K_{i_{left},j}$ for $j_* \leq j \leq j^*$.  By construction, the cells to the left of these, namely $K_{i_{left}-1,j}$, cannot be in $C_1$ except when $i_{left} = 1$.  However, even in this latter case, we can use the support condition as in Lemma~\ref{lemma:supp} to show $C_1$ and $C_2$ would be connected if there were both cells $K_{0,j}$ in $C_1$ and a cell $K_2 = K_{0,j_2}$ in $C_2$, yielding a contradiction.  Therefore, we can safely assume that the cells $K_{i_{left}-1,j}$ are not in $C_1$ for $j_* \leq j \leq j^*$.  Since $K_{i_{left}-1,j_*}$ is not in $C_1$, there exists at least one B\'ezier element $Q_L \equiv Q_{i_{left},j}$, with $j_*+1 \le j \le j_*+p$, within the support of its associated basis function such that it is contained in $\M_{\ell,\tilde Q}$ but not in $\Omega_{\ell+1}$.  We may repeat the same argument to show that $K_{i_{left},j_*-1}$ is not in $C_1$, and there is another element $Q_D \equiv Q_{i,j_*}$, with $i_{left}+1 \le i \le i_{left}+p$, within the support of the basis function associated with $K_{i_{left},j_*-1}$ such that it is in $\M_{\ell,\tilde Q}$ but not in $\Omega_{\ell+1}$. We have graphically depicted the previous steps of the proof in Figure~\ref{fig:point-i)} for the worst case configuration, in which the distance between the cells $K_{i_{left},j_*}$ and $K_{i_2,j_2}$ inside is the maximum possible.

\begin{figure}[ht]
%\begin{subfigure}[]{
\includegraphics[width=0.49\textwidth,trim=1cm 1cm 1cm 1cm, clip]{MG_qtilde_hatched}
%}
%\end{subfigure}
%\begin{subfigure}[]{
\includegraphics[width=0.49\textwidth,trim=1cm 1cm 1cm 1cm, clip]{MB_qtilde_hatched}
%}
%\end{subfigure}
%\includegraphics[width=\textwidth]{supports}
\caption{Graphical representation of the proof of Proposition~\ref{prop:cc}, with a configuration corresponding to degree $p=5$, as in Figure~\ref{fig:qtilde}. The Greville mesh $\MG'_{\ell,\tilde Q}$ is shown on the left, while on the right we show the B\'ezier submesh $\M_{\ell,\tilde Q}$. The two green diagonally hatched Greville cells in the left figure correspond to $K_{i_{left},j_*}$ (upper-right) and $K_{i_2,j_2}$ (bottom-left), while the supports of the associated 2-form basis functions, which are contained in $\Omega_{\ell+1}$, are also diagonally hatched in the right figure. The other two Greville cells correspond to $K_{i_{left}-1,j_*}$ (red vertically hatched) and $K_{i_{left},j_*-1}$ (red horizontally hatched), while on the right we have used the same pattern to draw the region of the support of the associated basis functions that is not completely contained in $\Omega_{\ell+1}$, and where the elements $Q_L$ and $Q_D$ lie. The purple element on the right corresponds to $Q_{i_{left},j_*}$, which is contained in $\Omega_{\ell+1}$. Finally, the blue vertex in the left figure is associated to a 0-form basis function, whose support is highlighted by the blue rectangle in the right figure. Since the diagonally hatched regions and $Q_{i_{left},j_*}$ are contained in $\Omega_{\ell+1}$, its overlap is not connected, which contradicts Assumption~\ref{ass:overlap}.}
\label{fig:point-i)}
\end{figure}

Now consider the basis function associated to the lower-left vertex of $K_{i_{left},j_*}$.  The support of this basis function subsumes the supports of the basis functions associated with cells $K_{i_{left}-1,j_*}$ and $K_{i_{left},j_*-1}$, thus the support contains both $Q_L$ and $Q_D$.  By Assumption ~\ref{ass:overlap}, it follows that $Q_{i_{left},j_*}$ must not be in $\Omega_{\ell+1}$, otherwise the overlap of the basis function associated to the lower-left vertex of $K_{i_{left},j_*}$ will not be connected (see Figure~\ref{fig:point-i)}).  This is in contradiction with the presence of a cell $K_2 \equiv K_{i_2,j_2}$ in $C_2$ with $0\le i_2 < i_{left}$ and $0 \le j_2 < j_*$ since the element $Q_{i_{left},j_*}$ belongs to the support of the basis function associated with this cell and therefore should be in $\Omega_{\ell+1}$.

We may repeat the same arguments as above to show that a contradiction arises if we assume that $i_2 > i_{right}$, $j_2 < j_{bottom}$, or $j_2 > j_{top}$.  Thus, we have arrived at the desired result.
\end{enumerate}
\end{proof}

We now prove the analogous result for the holes. Before proceeding, let us denote the complementary regions of the subdomains of interest by $\Omega^c_{\ell+1} := \Omega_0 \setminus \overline \Omega_{\ell+1}$, $\MG^c_{\ell,\ell+1} := \Omega_0 \setminus \overline \MG_{\ell,\ell+1}$ and $\MG^c_{\ell+1,\ell+1} := \Omega_0 \setminus \overline \MG_{\ell+1,\ell+1}$. Since we are in the planar two-dimensional case, we can define a hole of $\Omega_{\ell+1}$ as a connected component $\hole \subset \Omega^c_{\ell+1}$ such that $\partial \hole \cap \partial \Omega_0 = \emptyset$. The holes for the Greville subgrids are defined analogously.

\begin{proposition}\label{prop:holes}
The following statements hold:
\begin{enumerate}[i)]
\item Every hole of $\MG_{\ell+1,\ell+1}$ contains at least one hole of $\Omega_{\ell+1}$.
\item Every hole of $\MG_{\ell,\ell+1}$ contains at least one hole of $\MG_{\ell+1,\ell+1}$.
\item Under Assumptions~\ref{ass:support} and~\ref{ass:overlap}, every hole of $\MG_{\ell,\ell+1}$ contains exactly one hole of $\Omega_{\ell+1}$.
\item Under Assumptions~\ref{ass:support} and~\ref{ass:overlap}, every hole of $\Omega_{\ell+1}$ is contained in a hole of $\MG_{\ell,\ell+1}$.
\end{enumerate}
\end{proposition}
\begin{proof} We prove each statement independently.
\begin{enumerate}[i)]
\item As a consequence of point ii) in Proposition~\ref{prop:cc}, any connected component of $\Omega_{\ell+1}^c$ is contained in a connected component of $\MG^c_{\ell+1,\ell+1}$. Let $\hole^\MG \subset \MG^c_{\ell+1,\ell+1}$ be a hole, which is a connected component of $\MG^c_{\ell+1,\ell+1}$ with $\partial \hole^\MG \cap \partial \Omega_0 = \emptyset$.  Thus if $\hole^\MG$ contains a connected component of $\Omega_{\ell+1}^c$, that component must also be a hole. We will show that there is at least one.

Let us consider a function associated to a Greville cell in $\hole^\MG$. Since the cell is not in $\MG_{\ell+1,\ell+1}$, there exists at least one element $Q \in \M_{\ell+1}$ in the support of the associated basis function that is not contained in $\Omega_{\ell+1}$. As a consequence, $\MG_{\ell+1,\tilde Q} \subset \MG^c_{\ell+1,\ell+1}$, and by point ii) in Lemma~\ref{lemma:one-cell} and since $\MG_{\ell+1,\tilde Q}$ is connected, we have $Q \subset \MG_{\ell+1,\tilde Q} \subset \hole^\MG$, which proves the result.
\item Let $\hole^\MG_\ell \subset \MG^c_{\ell,\ell+1}$ be a hole. Reasoning as in point i), and using point i) in Proposition~\ref{prop:cc}, it is readily shown that any connected component of $\MG^c_{\ell+1,\ell+1}$ contained in $\hole^\MG_\ell$ must be a hole. To show that there is at least one, consider a Greville cell in $\hole^\MG_\ell$ and its associated basis function. The support of this function must contain an element $Q \subset \Omega^c_{\ell+1}$, and the function must have a child in ${\cal B}^2_{\ell+1}$ such that its support also intersects $Q$. The Greville cell associated with the child is in $\MG^c_{\ell+1,\ell+1}$, and it must be contained in $\MG_{\ell,\tilde Q} \subset \hole^\MG_\ell$.  This proves the result.
\item Assume that a hole $\hole^\MG \subset \MG^c_{\ell,\ell+1}$ contains more than one hole of $\Omega_{\ell+1}$. For each hole $\hole \subset \Omega_{\ell+1}^c$ we can consider a basis function in ${\cal B}^2_\ell$, with associated Greville cell in $\hole^\MG$, such that its support intersects $\hole$. Since $\hole^\MG$ is connected, we can construct a ``path'' of Greville cells in $\hole^\MG$ between the cells of two such functions corresponding to two different holes in $\Omega_{\ell+1}^c$. The support of every function associated to a Greville cell in this path intersects $\Omega_{\ell+1}^c$, and by Assumption~\ref{ass:overlap}, this intersection is contained in one connected component of $\Omega_{\ell+1}^c$. But since the holes are connected components, there exist two adjacent Greville cells such that the supports of the associated basis functions intersect two different connected components. Then, the support of the basis function in ${\cal B}^1_\ell$ associated to the intermediate edge intersects both, which is a contradiction with Assumption~\ref{ass:overlap}.  This proves the result.
\item Let $\hole \subset \Omega^c_{\ell+1}$ be a hole. Let us take all the B\'ezier elements in $\hole$ and define $\tilde \hole^\MG = \bigcup_{Q \subset \hole} \MG_{\ell,\tilde Q}$, which is connected and contained in $\MG^c_{\ell,\ell+1}$.  By Lemma~\ref{lemma:one-cell}, $\hole \subset \tilde \hole^\MG$. Consider the connected component of $\MG^c_{\ell,\ell+1}$ that contains $\tilde \hole^\MG$ which we henceforth denote as $\hole^\MG$. We want to prove that $\hole^\MG$ is a hole, that is, $\partial \hole^\MG \cap \partial \Omega_0 = \emptyset$.

Assume it is not true, i.e., there exists a Greville cell in $\hole^\MG$ adjacent to the boundary of $\Omega_0$. Since we are using an open knot vector, the support of the corresponding basis function is contained in B\'ezier elements adjacent to the boundary, and since the Greville cell is in $\hole^\MG \subset \MG^c_{\ell,\ell+1}$ and $\hole$ is a hole, one of these elements must be in $\Omega^c_{\ell+1}$ and contained in a connected component $\hole' \ne \hole$. Moreover, there exists a Greville cell in $\tilde \hole^\MG$ such that the support of the associated function in ${\cal B}^2_\ell$ intersects $\hole$, and reasoning as in point iii) we can build a path of Greville cells between this cell and the one adjacent to the boundary, which leads to a contradiction with Assumption~\ref{ass:overlap}, because $\hole$ and $\hole'$ are not connected.
\end{enumerate}
\end{proof}

The proof of Theorem~\ref{th:homology} is a direct consequence of Propositions~\ref{prop:cc} and~\ref{prop:holes}.

\begin{remark}
It is likely that the proof of Theorem~\ref{th:homology} can be simplified, and generalized to arbitrary dimension, with a more intelligent use of homology theory. All our attempts in this direction have failed due to the difficulties related to having three different grids defined on different subdomains. That is the reason why we restricted ourselves to the planar two-dimensional case.%, {\Rd and also the reason to the ``weird'' definition of hole.}
\end{remark}



%%%%%%%%%%%%%%%%%%%%%%%%%%%%%%%%%%%%%%%%%%%%%%%%%%%%%%%%%%%%
\section{Proof of Lemma~\ref{lemma:curves}, point ii)}\label{sec:appendixb}
%%%%%%%%%%%%%%%%%%%%%%%%%%%%%%%%%%%%%%%%%%%%%%%%%%%%%%%%%%%%

For the proof we can assume, without loss of generality, that $\Omega_{\ell+1}$ is connected. If it is not, the procedure of the proof can be applied to each connected component separately.

Let $\Gamma_0$ be the most external boundary of $\Omega_{\ell+1}$, and let $\Gamma_1, \ldots, \Gamma_{\nh}$ be the other connected components of the boundary. By Proposition~\ref{prop:holes}, the sets $\Gamma_0, \ldots, \Gamma_{\nh}$ are in a one-to-one correspondence with the boundaries $\Gamma^\MG_j$ in the Greville subgrid of Figure~\ref{fig:harmonic}. Let us denote by ${\bf x}_j \in \Gamma_j$ their respective lowermost (and leftmost) corners, and assume that the $\Gamma_j$ are ordered from the position of ${\bf x}_j$ starting from the lowermost and leftmost, moving first horizontally and then vertically. Since we are in the planar case, and $\Omega_{\ell+1}$ is a manifold with boundary from Lemma~\ref{lemma:omwb}, each $\Gamma_j$ is associated to a hole $\hole_j$. We define $\gamma_j$, for $j = 1, \ldots, \nh$, as the straight line that, starting from ${\bf x}_j$, goes downwards until it encounters another boundary $\Gamma_k$, with $0 \le k < j$. Recalling that ${\boldsymbol \zeta}^1_j$ are the generators of the first cohomology group for splines, $H^1(\Xhat_{\ell,\ell+1})$, to prove the result it is enough to show that:
\begin{enumerate}[a)]
\item $\displaystyle \int_{\gamma_j} {\boldsymbol \zeta}^1_j \cdot d{\bf s}> 0$, \quad for $j = 1, \ldots, \nh$,
\item $\displaystyle \int_{\gamma_j} {\boldsymbol \zeta}^1_k \cdot d{\bf s} = 0$, \quad for $1 \le j < k \le \nh$,
\end{enumerate}
since in this case the matrix given by the coefficients $\left\{\int_{\gamma_j} {\boldsymbol \zeta}^1_k \cdot d{\bf s} \right\}_{j,k=1}^{\nh}$ is a lower triangular matrix with positive diagonal entries and hence non-singular.

To prove a), let us consider a curve $\gamma_j$ and the associated harmonic function ${\boldsymbol \zeta}^1_j$ which is constructed as in Figure~\ref{fig:harmonic}. Note that the B\'ezier element above and to the right of ${\bf x}_j$ is not contained in $\Omega_{\ell+1}$.  Moreover, note the support of any basis function associated to a degree of freedom pointing upwards in Figure~\ref{fig:harmonic} (right) is contained in $\Omega_{\ell+1}$ and located above the aforementioned element.  Hence, such a basis function does not intersect $\gamma_j$. Alternatively, it is trivial to see that there is at least one function associated to a degree of freedom pointing downwards such that its support intersects $\gamma_j$. Since both $\gamma_j$ and the function are oriented downwards, we have obtained a).

To prove b), let us consider the same curve $\gamma_j$ but a different harmonic function ${\boldsymbol \zeta}^1_k$ with $k > j$ built as in Figure~\ref{fig:harmonic} for a different hole. From the ordering of $\Gamma_j$, and reasoning as in point a), the support of the functions associated to degrees of freedom pointing upwards cannot intersect $\gamma_j$. Assume now that there is at least one degree of freedom pointing downwards such that the support of its associated basis functions intersects $\gamma_j$. In this case, consider the Greville point above the chosen Greville edge, which is in $\Gamma^\MG_k \subset \partial \MG_{\ell,\ell+1}$, and its associated basis function, which is in $\Xhat^0_\ell$ but not in $\Xhat^0_{\ell,\ell+1}$. Obviously, the support of this function intersects the hole $\hole_k$, and since it contains the support of the function associated to the Greville edge, it also intersects $\gamma_j$. Finally, since $k > j$, from the ordering of the boundaries and the construction of $\gamma_j$, the support of this function must also intersect the hole $\hole_j$.  Since the holes are connected components of $\Omega_{\ell+1}^c$ this contradicts Assumption~\ref{ass:overlap}, which ends the proof.
